# Supplementary material for: Optimal Control for Open Quantum System in Circuit Quantum Electrodynamics
Source: arXiv:2412.20149 source file (2024-12-28)
Supplement: Supplementary file 1 [file SM.pdf]

# Supplementary Material:
# Optimal Control for Open Quantum System in Circuit Quantum Electrodynamics

Mo Zhou,[1,2] F. A. Cárdenas-López,[3,*] Sugny Dominique,[4] and Xi Chen[2,†]

[1] *Institute for Quantum Science and Technology, Department of Physics, Shanghai University, Shanghai 200444, China*
[2] *Instituto de Ciencia de Materiales de Madrid (CSIC), Cantoblanco, E-28049 Madrid, Spain*
[3] *Forschungszentrum Jülich GmbH, Peter Grünberg Institute, Quantum Control (PGI-8), 52425 Jülich, Germany*
[4] *Laboratoire Interdisciplinaire Carnot de Bourgogne, CNRS UMR 6303, Université de Bourgogne, BP, 47870, F-21078 Dijon, France*

(Dated: December 28, 2024)

This Supplementary Material provides detailed derivations supporting the main results. First, we derive the quantum Langevin equation (LE) and input-output theory, describing the dynamics of a single resonator in an open system. We show that, under coherent driving, the quantum LE is equivalent to the Lindblad formalism. Next, we apply the Pontryagin Maximum Principle (PMP) to find optimal control solutions for minimizing energy cost and operation time. We also derive counter-diabatic driving for open quantum systems and analyze their performance. Finally, we compare the signal-to-noise ratios (SNR) for various driving schemes, highlighting the advantages of the PMP-optimized pulses.

## I. QUANTUM LANGEVIN EQUATION, INPUT-OUTPUT THEORY AND MASTER EQUATION

In this section, we examine the system-bath interaction, describing the influence of the bath using equivalent input and output fields. We consider an open quantum system coupled to a heat bath, with the total Hamiltonian given by [1], $H_{\rm tot} = H_S + H_B + H_I$, where the system Hamiltonian, hereafter $\hbar = 1$, is $H_S = \omega_r a^\dagger a$, with $a$ and $a^\dagger$ being the annihilation (creation) operators for the system, $\omega_r$ the resonator frequency. The bath is modeled as a continuum of harmonic oscillators, $H_B = \int d\omega' \omega' b^\dagger(\omega') b(\omega')$ and the system-bath interaction is given by $H_I = i \int d\omega' \lambda(\omega')[b^\dagger(\omega') a - a^\dagger b(\omega')]$, where $b(\omega')$ and $b^\dagger(\omega')$ are the annihilation and creation operators and $\lambda(\omega')$ is the system-bath coupling strength. The equations of motion for $a$ and $b(\omega')$ are derived from the Heisenberg equation of motion, resulting in: $\dot{a} = -i[a, H_S] - i[a, H_I]$ and $\dot{b}(\omega') = -i[b(\omega'), H] = -i\omega' b(\omega') + \lambda(\omega') a$. Substituting $H_S$ and $H_I$ into the first equation for $\dot{a}$, we obtain

$$\dot{a} = -i\omega_r a - \int d\omega' \lambda(\omega') b(\omega'). \tag{1}$$

The equation for $b(\omega')$ is a first-order differential equation with the solution,

$$b(\omega') = e^{-i\omega' t} b_0(\omega') + \lambda(\omega') \int_0^t e^{-i\omega'(t-t')} a(t') dt', \tag{2}$$

where $b_0(\omega')$ is the initial value of the bath operator. Substituting this solution into Eq. (1), we obtain

$$\dot{a} = -i\omega_r a - \int d\omega' \lambda(\omega') \Big[ e^{-i\omega' t} b_0(\omega') + \lambda^*(\omega') \int_0^t e^{-i\omega'(t-t')} a(t') dt' \Big]. \tag{3}$$

Under the Markov approximation, assuming $\lambda(\omega')$ is frequency-independent, $\lambda(\omega') = \sqrt{\kappa/2\pi}$, and treating bath correlations as white noise, the integral $\int d\omega' e^{i\omega'(t-t')} = 2\pi\delta(t-t')$ helps us simplify the last term into $\kappa a/2$. By further defining the input noise operator as $a_{\rm in}(t) = (1/\sqrt{2\pi}) \int d\omega' e^{-i\omega' t} b_0(\omega')$, Eq. (3) becomes

$$\dot{a} = -i\omega_r a - \sqrt{\kappa} a_{\rm in}(t) - \frac{\kappa}{2} a. \tag{4}$$

When connecting the driving field to input field, $\varepsilon(t) = \sqrt{\kappa} a_{\rm in}(t)$, the quantum Langevin equation (LE) is finally obtained as

$$\dot{\alpha} = -i\omega_r \alpha - \frac{\kappa}{2}\alpha - \varepsilon(t), \tag{5}$$

where we use the expectation value $\langle a \rangle = \alpha(t)$, and the explicit time dependence of $\alpha(t)$ is omitted for simplicity. Similarly, considering a future time $t_\infty > t$ and the bath operator of that time $b_1(\omega')$, the solution for $b(\omega')$ changes to

$$b(\omega') = e^{-i\omega' t} b_1(\omega') + \lambda(\omega') \int_t^{t_\infty} e^{-i\omega'(t-t')} a(t') dt'. \tag{6}$$

We define the output field as $a_{\text{out}}(t) = \frac{1}{\sqrt{2\pi}}\int d\omega' e^{-i\omega' t} b_1(\omega')$. Following the same procedure, we derive the LE for the future time $t_\infty$:

$$\dot{a} = -i\omega_r a - \sqrt{\kappa}a_{\text{out}}(t) + \frac{\kappa}{2}a. \tag{7}$$

The input-output relation is given by

$$a_{\text{out}}(t) = a_{\text{in}}(t) + \sqrt{\kappa}a. \tag{8}$$

The connection between the quantum LE and the master equation has been rigorously established in Ref. [2] using the framework of quantum stochastic differential equations. Within the context of open quantum systems, the dynamics of a harmonic oscillator interacting with its environment are analyzed by deriving both the quantum LE and the Lindblad master equation from first principles. The quantum LE captures the system's dynamics by explicitly incorporating dissipation and quantum noise through operator-valued noise terms. In contrast, the master equation describes the time evolution of the system's density matrix, offering a statistical representation of the same underlying physical processes. Under the Markovian approximation, one can demonstrate the mathematical consistency and physical equivalence of these two approaches. This establishes a bridge between the microscopic, operator-based description of the quantum LE and the broader, ensemble-averaged perspective of the master equation, providing complementary insights into open system dynamics. To avoid unnecessary repetition, we directly present the master equation in the following form [2]:

$$\frac{d\rho}{dt} = i[\rho, H_S] + \frac{\kappa}{2}(2a^\dagger\rho a - \rho a a^\dagger - a a^\dagger\rho) - \sqrt{\kappa}[\rho, a^\dagger]a_{\text{in}}(t) + \sqrt{\kappa}[\rho, a]a^\dagger_{\text{in}}(t), \tag{9}$$

where the first term on the right-hand side describes the coherent evolution governed by the system Hamiltonian $H_S$, the second term accounts for dissipation from coupling to the environment and the last two terms capture the effects of the input noise field. Specifically, when consider the incoming noise field as coherent driving, e.g., $\varepsilon(t) = \sqrt{\kappa}a_{\text{in}}(t)$, we can rewrite the master equation for a driven harmonic oscillator in the presence of dissipation [3],

$$\frac{d\rho}{dt} = i[\rho, H'_S] + \frac{\kappa}{2}(2a\rho a^\dagger - \rho a^\dagger a - a^\dagger a\rho), \tag{10}$$

where the system Hamiltonian $H'_S$ takes the form

$$H'_S = \omega_r a^\dagger a + i(\varepsilon^*(t)a - \varepsilon(t)a^\dagger). \tag{11}$$

This formulation highlights the interplay between coherent evolution, dissipation, and external driving, offering a comprehensive framework for analyzing the dynamics of open quantum systems.

The coherent state of a harmonic oscillator can represent the density operator as $\rho(t) = |\alpha\rangle\langle\alpha|$. Its time derivative is expressed by $d\rho/dt = (\frac{d}{dt}|\alpha\rangle)\langle\alpha| + |\alpha\rangle\frac{d}{dt}\langle\alpha|$. Using the displacement operator, the first term becomes

$$\left(\frac{d}{dt}|\alpha\rangle\right)\langle\alpha| = \left(-\frac{1}{2}\frac{d|\alpha|^2}{dt} + \frac{\dot{\alpha}}{\alpha}a^\dagger a\right)|\alpha\rangle\langle\alpha|, \tag{12}$$

where the Baker-Campbell-Hausdorff formula $\exp(A+B) = \exp(-[A,B]/2)\exp(A)\exp(B)$ and the condition $a|0\rangle = 0$ are used. The second term $|\alpha\rangle d\langle\alpha|/dt$ is the Hermitian conjugate of the above. Thus, the left-hand side of the master equation (10) becomes

$$\frac{d\rho}{dt} = -\frac{d|\alpha|^2}{dt}|\alpha\rangle\langle\alpha| + \frac{\dot{\alpha}}{\alpha}a^\dagger a|\alpha\rangle\langle\alpha| + \frac{\dot{\alpha}^*}{\alpha^*}|\alpha\rangle\langle\alpha|a^\dagger a. \tag{13}$$

Next, consider the commutator $[\rho, H'_S]$, with Hamiltonian in Eq. (11):

$$[\rho, H'_S] = \left(\omega_r - i\frac{\varepsilon(t)}{\alpha^*}\right)|\alpha\rangle\langle\alpha|a^\dagger a - \left(\omega_r - i\frac{\varepsilon(t)}{\alpha}\right)a^\dagger a|\alpha\rangle\langle\alpha| + \varepsilon^*(t)(\alpha + \alpha^*)|\alpha\rangle\langle\alpha|, \tag{14}$$

the dissipation term is

$$\frac{\kappa}{2}(2a\rho a^\dagger - a^\dagger a\rho - \rho a^\dagger a) = \kappa|\alpha|^2|\alpha\rangle\langle\alpha| - \frac{\kappa}{2}a^\dagger a|\alpha\rangle\langle\alpha| - \frac{\kappa}{2}|\alpha\rangle\langle\alpha|a^\dagger a. \tag{15}$$

Comparing Eqs. (13-15), we derive the quantum LE using the coefficient of terms $a^\dagger a|\alpha\rangle\langle\alpha|$:

$$\frac{\dot{\alpha}}{\alpha} = -i\left(\omega_r - i\frac{\varepsilon(t)}{\alpha^*}\right) - \frac{\kappa}{2}, \tag{16}$$

which provides the earlier result (5). This demonstrates that a single harmonic oscillator coupled to an environment is equivalent to a driven harmonic oscillator with losses, as described by the quantum LE, provided the relation, $\varepsilon(t) = \sqrt{\kappa}a_{\text{in}}$.

## II. TIME AND ENERGY MINIMIZATION USING THE PMP METHOD

In this section, we outline a general method for optimizing driving field $\varepsilon(t)$, designed to drive the system from an initial configuration $\alpha(0)$ at $t = 0$ to a final one $\alpha(t_f)$ at $t = t_f$, while minimizing a relevant physical quantity. To begin, let us consider the following linear control problem:

$$\frac{\mathrm{d}\mathbf{x}}{\mathrm{d}t} = \hat{A}\,\mathbf{x} + \hat{B}\,\mathbf{u}(\mathbf{t}), \tag{17}$$

where $\mathbf{x}(t)$ represents the state of the system, and $\mathbf{u}(\mathbf{t})$ is the control vector. If the matrix $\hat{A}$ is time-independent, then the solution to this control problem (17) has the formal solution $\mathbf{x}(t) = \exp[\hat{A}t]\mathbf{x}(0) + \int_0^t \exp[\hat{A}(t-s)]\hat{B}\,\mathbf{u}(s)\mathrm{d}s$, where $\mathbf{x}(0)$ is the initial state. The control problem is subject to fixed boundary conditions: $\mathbf{x}(t_f) = \exp[\hat{A}t_f]\mathbf{x}(0) - \int_0^{t_f} \exp[\hat{A}(t-s)]\hat{B}\,\mathbf{u}(s)\mathrm{d}s$. We aim to minimize the functional, $J = \int f[\mathbf{x}, \mathbf{u}, t]dt$, where the additional constraints are incorporated into the optimization problem via the Pontryagin Maximum Principle (PMP).

For energy minimization, we define the cost function as: $J_E = \int_0^{t_f} \mathbf{u}^{\mathbf{T}}\mathbf{u}dt$. The Pontryagin Hamiltonian $H_c$ is given by: $H_c = \mathbf{u}^T\mathbf{u} + \mathbf{p}^T \cdot \dot{\mathbf{x}}$ where $\dot{\mathbf{x}}$ is derived from the linear equation, and the adjoint variable $\mathbf{p}$ is determined by the canonical equation $\dot{\mathbf{p}} = -\partial H_c/\partial \mathbf{x}$. To find the minimal energy cost, the control function must satisfy $\partial H_c/\partial \mathbf{u} = 0$. From this, we obtain the following conditions: $\dot{\mathbf{x}} = \hat{A}\mathbf{x} + \hat{B}\mathbf{u}$, $\dot{\mathbf{p}} = -\hat{A}^{\mathbf{T}}\mathbf{p}$, and $\mathbf{u} = \hat{B}^{\mathbf{T}}\mathbf{p}$. The formal solutions of the system are

$$\mathbf{x}(t) = e^{\hat{A}t}\mathbf{x}(0) + \int_0^t e^{\hat{A}(t-s)}\hat{B}\mathbf{u}ds, \tag{18}$$

$$\mathbf{p}(t) = e^{\hat{A}^{\mathbf{T}}(t_f - t)}\mathbf{p}(0), \tag{19}$$

where $\mathbf{x}(0)$ is the initial state and $\mathbf{p}(0)$ is the initial value. Then we can express the state as

$$\mathbf{x}(t) = e^{\hat{A}t}\mathbf{x}(0) + \int_0^t e^{\hat{A}(t-s)}\hat{B}\hat{B}^{\mathbf{T}}e^{A^{\mathbf{T}}(t-s)}ds\mathbf{p}(0). \tag{20}$$

The final condition $\mathbf{x}(t_f)$ allows us to determine $\mathbf{p}(0)$, that is,

$$\mathbf{p}(0) = \left[\int_0^{t_f} \exp[\hat{A}(t_f - s)]\hat{B}\hat{B}^{\mathbf{T}} \exp[\hat{A}^{\mathbf{T}}(t_f - s)]ds\right]^{-1} \left[\mathbf{x}(t_f) - \exp[\hat{A}t_f]\mathbf{x}(0)\right]. \tag{21}$$

Finally, the control vector is calcaulated as

$$\mathbf{u}^{\mathrm{opt}}(t) = \hat{B}^{\mathbf{T}} \exp[\hat{A}^{\mathbf{T}}(t_f - t)]\mathbf{p}(0). \tag{22}$$

This procedure is equivalent to the inverse-engineering method of the Lagrangian formalism by generalizing the approach commonly used to describe the superoscillation phenomenon [3]. Following the Lagrangian multiplier formalism, the optimization condition is

$$\frac{\partial J_E}{\partial \mathbf{u}(t)} - \hat{\mu}_0^T \frac{\partial \hat{G}_0[\mathbf{u}(t)]}{\partial \mathbf{u}(t)} = 0, \tag{23}$$

where $\hat{G}_0[\mathbf{u}(t)] = \int_0^{t_f} \exp[\hat{A}(t_f - s)]\hat{B}\mathbf{u}(s)ds - \mathbf{x}(t_f) + \exp[\hat{A}t_f]\mathbf{x}(0)$ is nothing but the boundary condition. To minimize the energy, we start with the functional: $J_E = \int_0^{t_f} \mathbf{u}^{\mathbf{T}}\mathbf{u}dt$. In this case, the control problem equation (23) becomes

$$\mathbf{u}^{\mathrm{opt}}(t) = 2\hat{B}^{\mathbf{T}} \exp[\hat{A}^{\mathbf{T}}(t_f - t)]\hat{\mu}_0. \tag{24}$$

Substituting the control vector $\mathbf{u}(t)$ into the boundary condition $\hat{G}_0[\mathbf{u}(t)] = 0$, we solve for the multiplier $\hat{\mu}_0$, corresponding to the Gramian matrix [4], yielding:

$$\hat{\mu}_0 = \frac{1}{2}\left[\int_0^{t_f} \exp[\hat{A}(t_f - s)]\hat{B}\hat{B}^{\mathbf{T}} \exp[\hat{A}^{\mathbf{T}}(t_f - s)]ds\right]^{-1} \left(\mathbf{x}(t_f) - \exp[\hat{A}t_f]\mathbf{x}(0)\right). \tag{25}$$

Thus, the control vector is

$$\mathbf{u}^{\mathrm{opt}}(t) = \hat{B}^{\mathbf{T}} \exp[\hat{A}^{\mathbf{T}}(t_f - t)]\left[\int_0^{t_f} \exp[\hat{A}(t_f - s)]\hat{B}\hat{B}^{\mathbf{T}} \exp[\hat{A}^{\mathbf{T}}(t_f - s)]ds\right]^{-1} \left[\mathbf{x}(t_f) - \exp[\hat{A}t_f]\mathbf{x}(0)\right]. \tag{26}$$

Compared this result with the PMP expression (22), we prove that both methods give the same optimal control, suggesting that the Lagrangian multiplier approach is equivalent to the PMP under the same conditions.

Now, to connect this control problem with the LE (5), we define $\alpha(t) = x_1(t) + ix_2(t)$ and $\varepsilon(t) = \varepsilon_1(t) + i\varepsilon_2(t)$, which gives the following system:

$$\begin{pmatrix} \dot{x}_1(t) \\ \dot{x}_2(t) \end{pmatrix} = \begin{pmatrix} -\frac{\kappa}{2} & \omega_r \\ -\omega_r & -\frac{\kappa}{2} \end{pmatrix} \begin{pmatrix} x_1(t) \\ x_2(t) \end{pmatrix} + \begin{pmatrix} -1 & 0 \\ 0 & -1 \end{pmatrix} \begin{pmatrix} \varepsilon_1(t) \\ \varepsilon_2(t) \end{pmatrix}. \tag{27}$$

From this comparison, we identify $\mathbf{x}^{\mathbf{T}}(t) = [x_1(t), x_2(t)]$ and $\mathbf{u}^{\mathbf{T}}(t) = [\varepsilon_1(t), \varepsilon_2(t)]$, along with the constant matrices $\hat{A}$ and $\hat{B}$. The real and imaginary parts of $\alpha(t)$ describe the evolution of the state in phase space. Specifically, the real part $x_1$ and the imaginary part $x_2$, represent the position and momentum coordinates, respectively, and are related to the quadrature components of the harmonic oscillator, e.g., $x_1(t) = x\sqrt{m\omega_r/2}$ and $x_2(t) = p/\sqrt{m\omega_r/2}$, with $m$ being the effective mass and $\omega_r$ being the resonator frequency. Using these matrices along with Eq. (26), we derive the optimal pulse

$$\mathbf{u}^{\mathrm{opt}}(t) = \frac{\kappa \exp[\kappa(t+t_f)]}{1-\exp[\kappa t_f]} \begin{bmatrix} \alpha(t_f)e^{i\omega_r(t-t_f)} + \alpha^*(t_f)e^{-i\omega_r(t-t_f)} \\ i\alpha(t_f)e^{i\omega_r(t-t_f)} - i\alpha^*(t_f)e^{-i\omega_r(t-t_f)} \end{bmatrix}. \tag{28}$$

The driving field $\varepsilon(t) = \varepsilon_1(t) + i\varepsilon_2(t)$ can be calculated as

$$\varepsilon^{\mathrm{opt}}(t) = \frac{2\kappa \exp[\kappa(t+t_f)]}{1-\exp[\kappa t_f]} \alpha^*(t_f)e^{-i\omega_r(t-t_f)}, \tag{29}$$

from which we finally calculate the corresponding energy cost

$$J_E^{\mathrm{opt}}(t_f) = \frac{4\kappa|\alpha(t_f)|^2}{1-e^{-\kappa t_f}} \xrightarrow{t_f\to\infty} 4\kappa|\alpha(t_f)|^2. \tag{30}$$

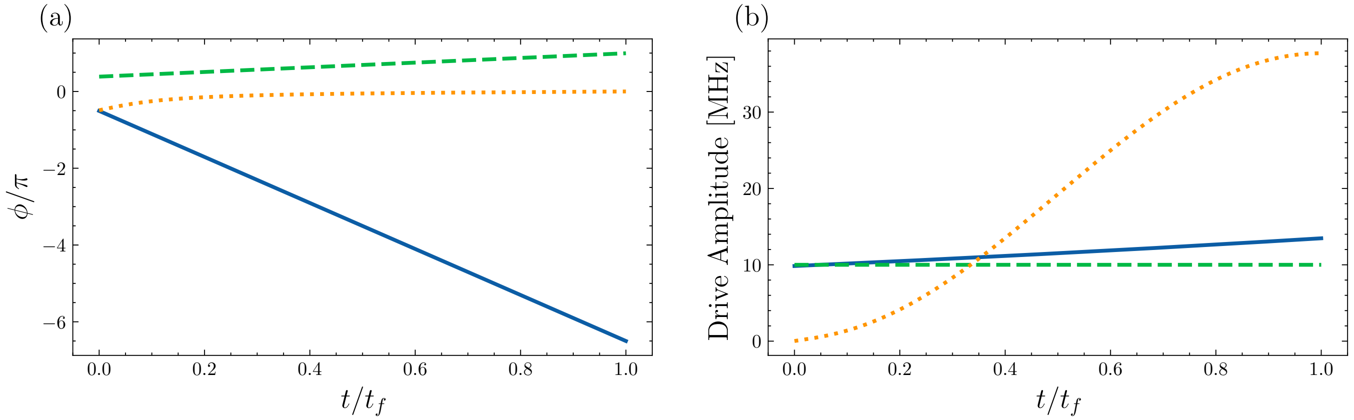


Figure S1. The phase (a) and amplitude (b) of the designed pulses are compared for three schemes: time-optimal (green dashed), energy-optimal (blue solid) and the CD driving (orange dotted). The energy-optimal pulse is designed with a fixed control $t_f$ = 10 µs, while the time-optimal pulse is constrained by a maximum driving amplitude of $\varepsilon_{\max}$ = 10 MHz, resulting in a minimal time of $t_f^{\min}$ = 1.01 µs. All three protocols successfully steer the system from the initial state $\alpha(0) = 0$ to the target state $\alpha(t_f) = 10e^{i\vartheta}$ at their respective final times. Other parameters: $\omega_r = 2\pi \times 0.3$ MHz and $\kappa = 2\pi \times 10$ kHz.

For a time-optimal driving field $\varepsilon(t)$, we aim to drive the system to the same target state with possible shortest time, while ensuring the maximum amplitude constraint $|\varepsilon(t)|^2 \le \varepsilon_{\max}$. This constraint allows us to parametrize the real and imaginary components of the pulse as $\varepsilon_1(t) = \varepsilon_{\max}\cos\phi(t)$, $\varepsilon_2(t) = \varepsilon_{\max}\sin\phi(t)$ [5], where $\phi(t)$ is a time-dependent function to be determined. In this manner, we simplify two control parameters to one control parameter. The LE for this case becomes:

$$\begin{pmatrix} \dot{x}_1(t) \\ \dot{x}_2(t) \end{pmatrix} = \begin{pmatrix} -\frac{\kappa}{2} & \omega_r \\ -\omega_r & -\frac{\kappa}{2} \end{pmatrix} \begin{pmatrix} x_1(t) \\ x_2(t) \end{pmatrix} + \begin{pmatrix} -\varepsilon_{\max} & 0 \\ 0 & -\varepsilon_{\max} \end{pmatrix} \begin{pmatrix} \cos\phi(t) \\ \sin\phi(t) \end{pmatrix}. \tag{31}$$

We can compute the minimal control time $J_T \equiv \int_0^{t_f} dt = 1$ using the PMP. Our aim is to find the time-optimal solution of $\varepsilon(t)$, more specifically $\phi(t)$, under the boundary conditions $\alpha(0)$ and $\alpha(t_f)$ with physical constraint $|\varepsilon(t)|^2 \le \varepsilon_{\max}$. The Pontryagin Hamiltonian is defined as $H_c = p_0 + \sum p_j\dot{x}_j$, where $p_0$ is the energy offset and $\dot{x}_j$ follows the LE, see Eq. (31). The adjoint

variables $(p_1, p_2)$ can be calculated using the canonical equations:

$$\begin{aligned} \dot{p}_1 &= -\frac{\partial H_c}{\partial x_1} = \frac{\kappa}{2} p_1 - \omega_r p_2, \\ \dot{p}_2 &= -\frac{\partial H_c}{\partial x_2} = \omega_r p_1 + \frac{\kappa}{2} p_2, \end{aligned} \tag{32}$$

from which the general solution evolves

$$\begin{aligned} p_1 &= e^{-\frac{\kappa t}{2}} [p_1(0)\cos(\omega_r t) - p_2(0)\sin(\omega_r t)], \\ p_2 &= e^{-\frac{\kappa t}{2}} [p_2(0)\cos(\omega_r t) + p_1(0)\sin(\omega_r t)]. \end{aligned} \tag{33}$$

We observe that $e^{\frac{\kappa t}{2}}(p_1^2 + p_2^2) = p_1^2(0) + p_2^2(0) = C^2$, which is constant. This conservation law allows us to express the initial conditions as $p_1(0) = C\cos\theta$, $p_2(0) = C\sin\theta$. According to PMP, to minimize the control time, we need to maximize the Pontryagin Hamiltonian. This leads to the condition $\partial H_c/\partial\phi = 0$, yielding $p_1\varepsilon_{\max}\sin\phi(t) - p_2\varepsilon_{\max}\cos\phi(t) = 0$, that means $\tan\phi = p_2/p_1$. Using the solution (33) and the initial conditions for $p_j$, we further get

$$\tan\phi^{\text{opt}}(t) = \frac{\cos\theta\cos(\omega_r t) - \sin\theta\sin(\omega_r t)}{\sin\theta\cos(\omega_r t) + \cos\theta\sin(\omega_r t)}, \tag{34}$$

which can be rewritten as $\phi^{\text{opt}}(t) = \omega_r t + \theta$. To determine the minimal time $t_f^{\min}$ and constant $\theta$, we solve for $\alpha(t)$ under the boundary conditions $\alpha(0)$ and $\alpha(t_f)$. To do this, we solve the LE with $\phi^{\text{opt}}(t)$ and obtain the solution for $\alpha^{\text{opt}}(t)$,

$$\alpha^{\text{opt}}(t) = \alpha(0)e^{-(\frac{\kappa}{2}+i\omega_r)t} + \frac{2\varepsilon_{\max}e^{i\theta}}{\kappa + 4i\omega_r}\left[e^{-(\frac{\kappa}{2}+i\omega_r)t} - 1\right]. \tag{35}$$

By setting the initial boundary condition $\alpha^{\text{opt}}(0) = 0$, we can solve for the minimal time $t_f^{\min}$ by ensuring that absolute value $|\alpha^{\text{opt}}(t_f^{\min})|$ matches the final boundary condition $|\alpha(t_f)|$. Once the minimal time $t_f^{\min}$ is obtained, the phase $\theta$ of the driving can be determined by satisfying the phase of $\alpha^{\text{opt}}(t_f^{\min})$ with that of final state $\alpha(t_f)$.

For the qubit-resonator interaction system, we use the same optimal solutions. The LE is modified as

$$\dot{\alpha} = -i\chi_z\alpha - \frac{\kappa}{2}\alpha - \varepsilon(t), \tag{36}$$

where the difference from the previous results is $\omega_r \to \chi_z$ and $\chi_z = \pm\chi$ is state-dependent Stark-shift. In this scenario, we obtain the optimal control for energy minimization as

$$\mathbf{u}^{\text{opt}}(t) = \frac{\kappa\exp[\kappa(t+t_f)]}{1-\exp[\kappa t_f]}\begin{bmatrix} \alpha(t_f)e^{i\chi_z(t-t_f)} + \alpha^*(t_f)e^{-i\chi_z(t-t_f)} \\ i\alpha(t_f)e^{i\chi_z(t-t_f)} - i\alpha^*(t_f)e^{-i\chi_z(t-t_f)} \end{bmatrix}, \tag{37}$$

and, for time minimization, the minimal time $t_f^{\min}$ with the same constraint is determined by

$$\alpha^{\text{opt}}(t_f^{\min}) = e^{-(\frac{\kappa}{2}+i\chi_z)t_f^{\min}} + \frac{2\varepsilon_{\max}e^{i\theta}}{\kappa + 4i\chi_z}\left[e^{-(\frac{\kappa}{2}+i\chi_z)t_f^{\min}} - 1\right]. \tag{38}$$

Now we present the energy-optimal and time-optimal controls for the dissipative oscillator system. Fig. S1 illustrates the amplitudes and phases of the driving schemes: the solid blue line represents the energy-optimal pulse, while the green dashed line corresponds to the time-optimal pulse, constrained by a maximum amplitude $\varepsilon_{\max}$. Additionally, Fig. S2 shows the phase (a) and amplitude (b) profiles of the designed driving pulses in the qubit-resonator interaction system. In these examples, the initial state is $\alpha(0) = 0$ and the final state is $\alpha(t_f) = 10e^{i\vartheta}$, with the fixed phase $\vartheta = \pi/2 + \arctan(\kappa/2\omega_r)$, as described below.

## III. COUNTERDIABATIC DRIVING

In this section, we will introduce the counter-diabatic (CD) driving for single resonator in open system. This concept was applied and experimentally verified in [6]. The dynamics of a single oscillator interacting with environment is described by the quantum LE:

$$\dot{\alpha} = -i\omega_r\alpha - \frac{\kappa}{2}\alpha - \varepsilon(t). \tag{39}$$

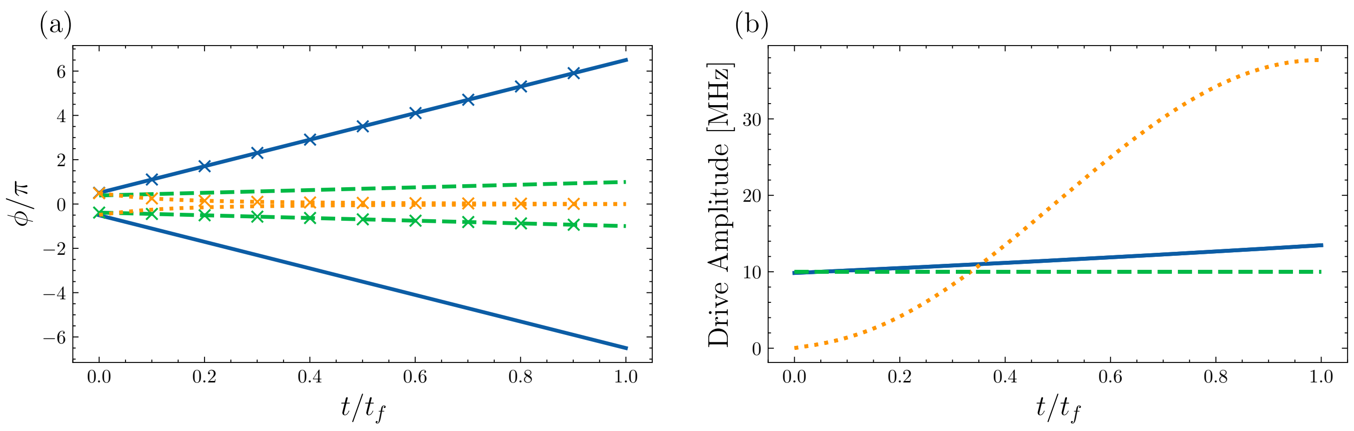


Figure S2. The phase (a) and amplitude (b) of three driving pulses are illustrated for the qubit-resonator interaction, which include the energy-optimal (blue solid), time-optimal (green dashed), and the CD driving (orange dotted). For the two distinct qubit states $|e\rangle$ and $|g\rangle$, the pulse amplitudes remain the same, whereas the phases are different. The phases corresponding to $|e\rangle$ are marked with crosses for distinction. Parameters: $\omega_r = 2\pi \times 6$ GHz, $\omega_q = 2\pi \times 4$ GHz, $\kappa = 2\pi \times 10$ kHz, and the rest are the same as those in Fig. S1.

The goal of CD driving is to introduce an auxiliary control added to the adiabatic reference to suppress undesired diabatic transitions when we accelerate the state evolution. In the adiabatic approximation, the system reaches the instantaneous equilibrium state $\bar{\alpha}$,

$$\bar{\alpha}(t) = \frac{i\varepsilon(t)}{\omega_r - i\kappa/2}. \tag{40}$$

when $\dot{\alpha} = 0$ in Eq. (39). By defining the instantaneous diabatic excitation as $\delta(t) = \alpha(t) - \bar{\alpha}(t)$, the dynamics of $\delta(t)$ is determined by

$$\dot{\delta}(t) = -i(\omega_r - i\kappa/2)\delta(t) - \varepsilon_{CD}(t) + \left(\varepsilon(t) - i\frac{\dot{\varepsilon}(t)}{\omega_r - i\kappa/2}\right). \tag{41}$$

Using the conditions to eliminate excitation, $\delta(t) = 0$ and $\dot{\delta}(t) = 0$, the desired CD driving is obtained as

$$\varepsilon_{CD}(t) = \varepsilon(t) - i\frac{\dot{\varepsilon}(t)}{\omega_r - i\kappa/2}. \tag{42}$$

As an example, we consider a Hahn pulse $\varepsilon_h(t) = \Omega_0 \sin^2(\pi t/2t_f)$ as an adiabatic reference, from which the corresponding CD driving pulse can be derived as

$$\varepsilon_{CD}(t) = \Omega_0 \sin^2(\pi t/2t_f) - i\frac{\pi\Omega_0 \sin(\pi t/2t_f)\cos(\pi t/2t_f)}{(\omega_r - i\kappa/2)t_f}. \tag{43}$$

Under the CD driving, the system dynamics follow

$$\alpha(t) = \bar{\alpha}(t) = \frac{i\Omega_0 \sin^2(\pi t/2t_f)}{\omega_r - i\kappa/2}, \tag{44}$$

leading to the final boundary condition

$$\alpha(t_f) = \frac{i\Omega_0}{\omega_r - i\kappa/2} = \frac{\Omega_0}{\sqrt{\omega^2 + \kappa^2/4}} e^{i\vartheta}, \tag{45}$$

where $\vartheta = \pi/2 + \arctan(\kappa/2\omega_r)$. In this case, using a Hahn pulse with real $\Omega_0$, the target state is chosen as $\alpha(t_f) = 10e^{i\vartheta}$. And the final coherent state can be expressed as $\alpha(t_f) = x_1(t_f) + ix_2(t_f)$, under the condition $x_1(t_f)/x_2(t_f) = \kappa/2\omega_r$. For comparison, Fig. S1 includes the CD-assisted pulse, represented by the orange dotted line, where the adiabatic Hahn pulse is expressed as $\varepsilon_h(t) = \Omega_0 \sin^2(\pi t/2t_f)$, with $\Omega_0 = |\alpha(t_f)|\sqrt{\omega_r^2 + \kappa^2/4}$ and $|\alpha(t_f)| = 10$. Notably, the CD driving yields a significantly larger pulse amplitude compared to the other optimal pulses, while achieving the same target state within the same time $t_f$.

Furthermore, we extend the concept of CD driving to the qubit-resonator interaction scenario. In this case, the CD driving is defined by substituting $\omega_r$ with $\chi_z = \pm\chi$ in Eq. (42). The resulting expression is

$$\varepsilon_{CD}(t) = \varepsilon(t) - i\frac{\dot{\varepsilon}(t)}{\chi_z - i\kappa/2}. \tag{46}$$

To compute the CD driving, we adopt the Hahn pulse used previously. Substituting this into Eq. (46), the CD driving becomes

$$\varepsilon_{CD}(t) = \Omega_0 \sin^2(\pi t/2t_f) - i\frac{\pi\Omega_0 \sin(\pi t/2t_f)\cos(\pi t/2t_f)}{(\chi_z - i\kappa/2)t_f}, \tag{47}$$

where $\Omega_0$ is determined earlier. Fig. S2 shows the phase (a) and amplitude (b) profiles of the CD driving pulses in the qubit-resonator interaction system.

For the two qubit states, $|e\rangle$ and $|g\rangle$, the pulse amplitudes are identical, but their phases differ. To emphasize this difference, the phases corresponding to the $|e\rangle$ state are marked with crosses in Fig. S2. In the main text and subsequent comparisons, the optimal pulses and CD driving for the qubit-resonator coupling system are computed using $\chi_z = \chi$. However, the alternative solutions, corresponding to $\chi_z = -\chi$, are equally valid. The main difference between these cases lies in the orientation of the pointer states in phase space. Notably, the qubit state $|e\rangle$ is more prone to relaxation and decoherence compared to $|g\rangle$. As such, employing the CD driving and optimal pulses tailored for $|e\rangle$ provides a significant advantage in achieving higher readout fidelity. Importantly, the sign of $\chi_z = \pm\chi$ does not affect the signal-to-noise ratio (SNR) because the SNR depends quadratically on $\chi_z$. However, when the qubit is in an undesired state, the optimal pulses and CD driving designed for the $|e\rangle$ state might require additional investigation to ensure performance. For further details, refer to the Supplementary Material in Ref. [6].

## IV. COMPARISON OF SNR FOR DIFFERENT DRIVINGS

In this section, we present a comprehensive comparison of the SNR for various driving schemes, while the main text focuses specifically on the optimal pulse for energy minimization. The SNR is defined as the ratio between the homodyne signal and its fluctuations, namely,

$$\text{SNR} = \frac{|\langle\hat{\mathcal{M}}_{|e\rangle}\rangle - \langle\hat{\mathcal{M}}_{|g\rangle}\rangle|}{\sqrt{\langle\hat{\mathcal{M}}^2_{\text{N}|e\rangle}\rangle + \langle\hat{\mathcal{M}}^2_{\text{N}|g\rangle}\rangle}}. \tag{48}$$

Here the homodyne signal is given by $|\langle\hat{\mathcal{M}}_{|e\rangle}\rangle - \langle\hat{\mathcal{M}}_{|g\rangle}\rangle|$ and the noise homodyne operator is defined by $\hat{\mathcal{M}}_{\text{N}|\ell\rangle} = \hat{\mathcal{M}}_{|\ell\rangle} - \langle\hat{\mathcal{M}}_{|\ell\rangle}\rangle$, where the average homodyne signal for the state $|\ell\rangle \in \{|g\rangle, |e\rangle\}$ is defined as $\hat{\mathcal{M}}_{|\ell\rangle}(\tau) = \sqrt{\kappa}\int_0^\tau dt[a^\dagger_{\text{out}}(t)\exp(i\varphi) + a_{\text{out}}(t)\exp(-i\varphi)]$. The output field $a_{\text{out}}(t)$ is determined by the input-output relation $a_{\text{out}}(t) = a_{\text{in}}(t) + \sqrt{\kappa}a$, and we can obtain $\alpha_{\text{out}}(t)$ as

$$\alpha_{\text{out}}(t) \equiv \langle a_{\text{out}}(t)\rangle = \sqrt{\kappa}e^{\kappa t/2 + i\chi_z t}\int_0^t \varepsilon(s)e^{-\kappa s/2 - i\chi_z s}ds, \tag{49}$$

by solving the LE (5). To evaluate the quality of the readout process, we calculate the SNR for other drivings, with $\varphi = 0$. As shown in Fig. S3(a), our energy-optimal control achieves higher SNR in a shorter time, evidenced by the rapid ascent of the solid lines compared to other schemes.

Additionally, we calculate the different SNR under the time-optimal control. It is important to note that reducing the maximum driving amplitude naturally leads to an increase in the shortest achievable time. This, in turn, results in more intricate trajectories during the readout process. The underlying reason lies in the trigonometric driving function $e^{i(\chi_z t+\theta)}$ in Eq. (38). If the control time extends significantly, the driving oscillation will encompass more than one cycle. To optimize the SNR, we can explore different measurement quadratures, see Fig. S3(b). The findings indicate that the SNR achieves its maximum value when the measurement angle $\varphi$ is an integer multiple of $\pi$.

* f.cardeans.lopez@fz-juelich.de
† xi.chen@csic.es

[1] H.-P. Breuer and F. Petruccione, *The theory of open quantum systems* (Oxford University Press, USA, 2002).
[2] C. W. Gardiner and M. J. Collett, Input and output in damped quantum systems: Quantum stochastic differential equations and the master equation, Phys. Rev. A **31**, 3761 (1985).

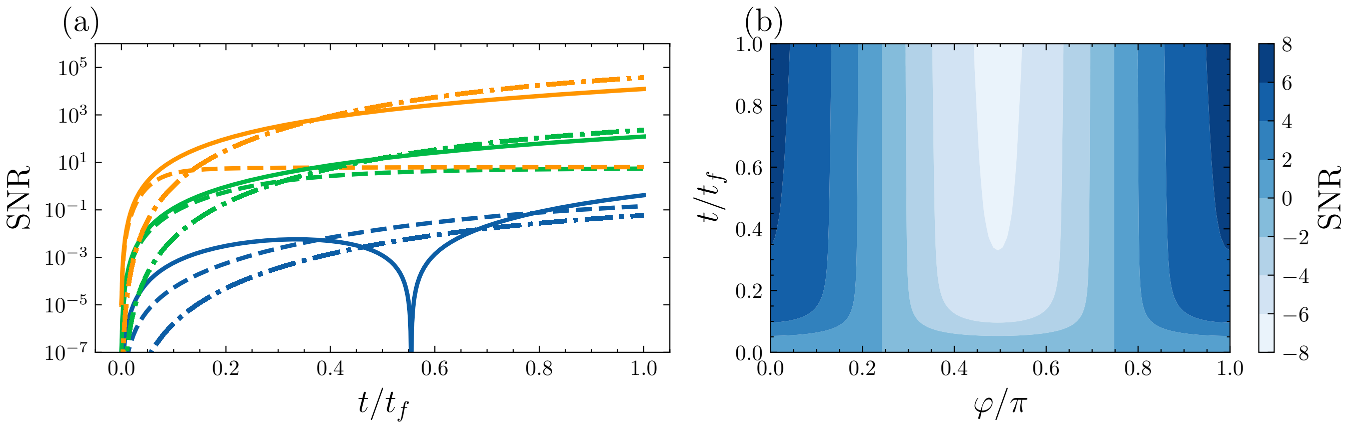


Figure S3. (a) The SNR results for three driving schemes with $\varphi = 0$ are displayed: energy-optimal (solid line), time-optimal (dashed line), and CD driving (dot-dashed line). Different colors represent different critical photon numbers: blue for $\bar{n}_{\rm crit} = 1$, green for $\bar{n}_{\rm crit} = 10$, and orange for $\bar{n}_{\rm crit} = 100$. All other parameters are identical to those in Fig. S2. (b) The contour map illustrates the influence of measurement angles $\varphi$ in the operator $\hat{\mathcal{M}}_{|\ell\rangle}$ and the evolution time on the SNR function.

[3] Q. Zhang, X. Chen, and D. Guéry-Odelin, Robust control of linear systems and shortcut to adiabaticity based on superoscillations, Phys. Rev. Appl. **18**, 054055 (2022).
[4] U. Boscain, M. Sigalotti, and D. Sugny, Introduction to the pontryagin maximum principle for quantum optimal control, PRX Quantum **2**, 030203 (2021).
[5] E. Dionis and D. Sugny, Time-optimal control of two-level quantum systems by piecewise constant pulses, Phys. Rev. A **107**, 032613 (2023).
[6] Z. Yin, C. Li, J. Allcock, Y. Zheng, X. Gu, M. Dai, S. Zhang, and S. An, Shortcuts to adiabaticity for open systems in circuit quantum electrodynamics, Nature Communications **13**, 188 (2022).
